# Supplementary material for: Classification of Endoscopy and Video Capsule Images using CNN-Transformer Model
Source: arXiv:2408.10733 source file (2024-08-20)
Supplement: Supplementary file 1 [file Supplementary.pdf]

# Classification of Endoscopy and Video Capsule Images using CNN-Transformer Model

Aliza Subedi[1], Smriti Regmi[1], Nisha Regmi[2], Bhumi Shankar Bhusal[2], Ulas Bagci[2], and Debesh Jha[2]

[1] Pashchimanchal Campus, Nepal
[2] Machine & Hybrid Intelligence Lab, Department of Radiology, Northwestern University, Chicago, USA

## 1 Dataset description

### 1.1 Gastrovision

The 23 classes from the Gastrovision dataset comprise a total of 7,930 images. These include 1,476 images for normal mucosa and vascular patterns in the large bowel, 1,266 for tools, 969 for the stomach, 820 for colon polyps, 846 for the small bowel terminal ileum, and 205 for the duodenal bulb. Additionally, there are 200 images of the ileocecal valve, 171 of blood in the lumen, 141 of dyed-lifted polyps, 246 of dyed-resection margins, 393 of the pylorus, 139 of colorectal cancer cases, and 330 of gastroesophageal and normal z-line junctions. Also included are 140 images of the normal esophagus, 113 of the cecum, 107 of esophagitis, 95 of Barrett's esophagus, 92 of resected polyps, 67 of the retroflex rectum, and 65 of gastric polyps. Lastly, the classes "Mucosal inflammation large bowel" and "Colon diverticula" each have 29 instances.

### 1.2 Kvasir-Capsule

This video capsule endoscopy dataset comprises 44,228 labeled images across 13 anatomical and luminal findings. We focused on 11 of these classes for analysis. The dataset reveals considerable class imbalance across its categories. Notably, the Pylorus class is represented by 1529 images, while the Ileocecal Valve class contains 4189 images, and the Ampulla of Vater class is notably sparse with only 10 images. Additionally, other classes include 34,338 images of Normal Clean Mucosa, 2906 of Reduced Mucosal View, 592 of Lymphangiectasia, 159 of Erythema, 866 of Angiectasia, 446 of Blood-Fresh, 12 of Blood-Hematin, 506 of Erosion, 854 of Ulcer, 55 of Polyp, and 776 of Foreign body. This diversity in image counts presents a challenge in training and evaluating machine learning models, necessitating strategies to address class imbalance effectively.

## 2 Visualization using saliency map

The saliency map created using the hybrid model trained on the Kvasir-Capsule dataset is presented in Figure 1. The Figure shows the significant regions in the input image that contribute to the model's decision.

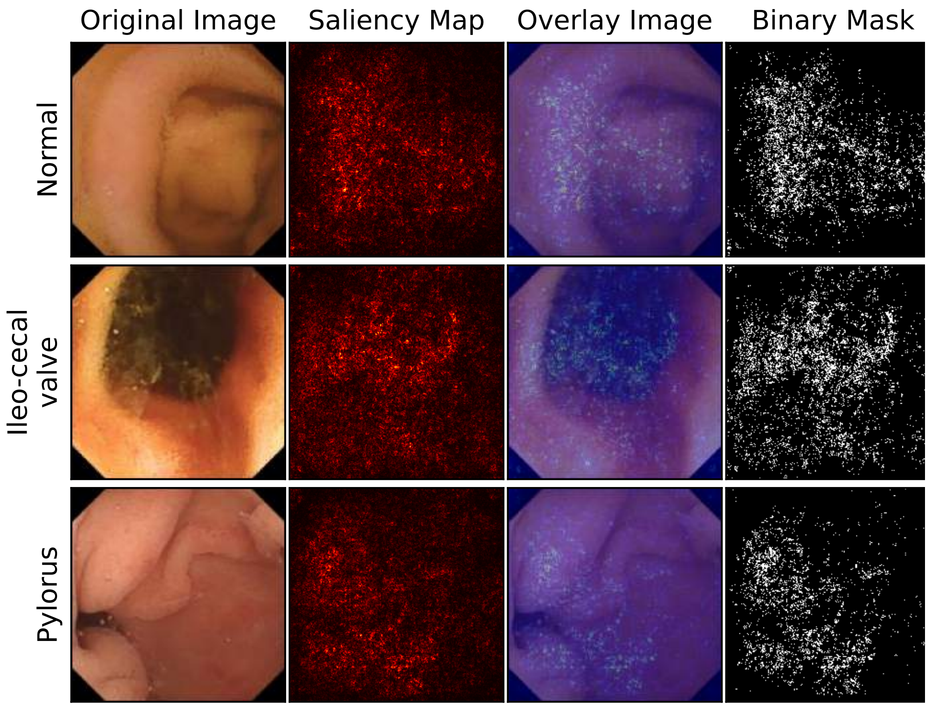


**Fig. 1:** Saliency maps visualization for Kvasir-Capsule dataset for three representative classes.
